# Supplementary material for: On-Shell Flow
Source: arXiv:2211.04231 source file (2022-11-08)
Supplement: Supplementary file 2 [file appendixB.tex]

Let's consider a metric flow source 
\be
\begin{split}
         A_{\mu\nu}&\equiv -2R_{\mu\nu}+2\vartheta Rg_{\mu\nu}+ b\nabla_\mu\nabla_\nu\phi+g_{\mu\nu}d\Delta\phi\\
     &\quad+e\nabla_\mu\phi\nabla_\nu\phi+fg_{\mu\nu}\nabla_\alpha\phi\nabla^\alpha\phi\ ,
\end{split}
\ee
as presented in \eqref{singsource}. Furthermore, following the discussion developed in \ref{singlesc}, let's impose $\vartheta=0$ and $b$, $d$, $e$ and $f$ to satisfy:
\be 
\begin{split}
    b=-2\left(1+2\gamma\right)\ ,\quad d=-f=2\left(1-\alpha-\frac{\gamma}{2}\right)\ ,\quad e=2\left(1-\alpha+\gamma\right)\ .
\end{split}
\ee
Given such expressions, one can simply derive:
\be 
e=d-\frac{3\left(2+b\right)}{4}\ .
\ee
From the construction of the $\mathcal{F}$-functional, one can obtain
\be
\begin{split}
    E_{\mu\nu}&=-\nabla_\mu\phi\nabla_\nu R+f_D\nabla_\mu\phi\nabla_\nu\left(\nabla\phi\right)^{2}-g_D\nabla_\mu\phi\nabla_\nu\Delta\phi\\
    &\quad-\nabla_\nu\phi\nabla_\mu R+f_D\nabla_\nu\phi\nabla_\mu\left(\nabla\phi\right)^{2}-g_D\nabla_\nu\phi\nabla_\mu\Delta\phi\\
    &\quad-g_{\mu\nu}m^2\phi\left[-R+f_D\left(\nabla\phi\right)^{2}-g_D\Delta\phi\right]\\
    &\quad+g_{\mu\nu}\left[\nabla^\alpha\phi\nabla_\alpha R+\frac{3}{4}\nabla^\alpha\phi\nabla_\alpha\left(\nabla\phi\right)^{2}+g_D\nabla^\alpha\phi\nabla_\alpha\Delta\phi\right]\\
    &\quad+2R_{\mu\nu}\left(\frac{1}{2}\nabla_\alpha\phi\nabla^\alpha\phi+\frac{m^2}{2}\phi^2\right)\\
    &\quad- b\nabla_\mu\nabla_\nu\phi\left(\frac{1}{2}\nabla_\alpha\phi\nabla^\alpha\phi+\frac{m^2}{2}\phi^2\right)\\
    &\quad-g_{\mu\nu}d\Delta\phi\left(\frac{1}{2}\nabla_\alpha\phi\nabla^\alpha\phi+\frac{m^2}{2}\phi^2\right)\\
    &\quad-\frac{2+4d+b}{4}\nabla_\mu\phi\nabla_\nu\phi\left(\frac{1}{2}\nabla_\alpha\phi\nabla^\alpha\phi+\frac{m^2}{2}\phi^2\right)\\
         &\quad+dg_{\mu\nu}\nabla_\alpha\phi\nabla^\alpha\phi\left(\frac{1}{2}\nabla_\alpha\phi\nabla^\alpha\phi+\frac{m^2}{2}\phi^2\right)\ ,
\end{split}
\ee
where we have defined:
\be 
\begin{split}
    f_D&\equiv\frac{4d-b-2}{8}\left(1-D\right)-\frac{b+2}{4}\left(1+\frac{D}{2}\right)\ ,\\
    g_D&\equiv 1-D\frac{4d-b-2}{8}-\frac{b+2}{4}\left(2+\frac{D}{2}\right)\ .
\end{split}
\ee
On the other hand, imposing the equations of motion to be on-shell we get
\be
\begin{split}
   2B_{\mu\nu}&=-2\nabla^\sigma\nabla_\nu R_{\mu\sigma}+2\nabla_\mu\nabla_\nu R+2\Delta R_{\mu\nu}\\
&\quad-2\nabla_\mu\nabla^\sigma R_{\sigma\nu}-g_{\mu\nu}\Delta R\\
    &\quad+2R_\mu{}^\sigma{}_\nu {}^\theta R_{\sigma\theta}+2RR_{\mu\nu}-2R_\mu{}^\sigma R_{\sigma\nu}-4\Lambda R_{\mu\nu}\\
    &\quad+2\left(C-R_{\sigma\theta}R^{\sigma\theta}\right)g_{\mu\nu}+\Omega_{\mu\nu}\phi\\
    &\quad     +\Theta_{\mu\nu}\nabla_\alpha\phi\nabla^\alpha\phi+\Sigma_{\mu\nu}^{\sigma\theta}\nabla_\sigma\phi\nabla_\theta\phi\ ,
\end{split}
\ee
where we have introduced
\be 
\begin{split}
    \Omega_{\mu\nu}&= b\nabla_\mu\Delta\nabla_\nu-\left[\left(D-2\right)d+b\right]\nabla_\mu\nabla_\nu\Delta- b\Delta\nabla_\mu\nabla_\nu\\
    &\quad+ \left[b\left(2\Lambda\delta_\mu{}^\sigma\delta_\nu{}^{\theta}+g_{\mu\nu}R^{\sigma\theta}\right)\nabla_\sigma\nabla_\theta\right]+ b\nabla^\sigma\nabla_\nu \nabla_\mu\nabla_\sigma\\
    &\quad+g_{\mu\nu}\left\{\left[\left(D-2\right)d+b\right]\Delta\Delta-b\nabla^\sigma\nabla^\theta\nabla_\sigma\nabla_\theta+2d\Lambda\Delta\right\}\\
    &\quad+\left[\left(R_\mu{}^\sigma\delta_\nu{}^{\theta}-R_\mu{}^\sigma{}_\nu {}^\theta-R\delta_\mu{}^\sigma\delta_\nu{}^{\theta}\right) b\nabla_\sigma\nabla_\theta\right]\ ,
\end{split}
\ee
\be
\begin{split}
   \Theta_{\mu\nu}&\equiv\left(g_{\mu\nu}\Delta-\nabla_\mu\nabla_\nu \right)\left[d\left(1-D\right)-\frac{3\left(2+b\right)}{4}\right]\\
   &\quad-2\left(\nabla_\mu\nabla_\nu-g_{\mu\nu}\Delta+\Lambda g_{\mu\nu}\right)d\ , 
\end{split}
\ee
and
\be
\begin{split}
   \Sigma_{\mu\nu}^{\sigma\theta}&\equiv \Big[\left(R_\mu{}^\sigma+\nabla_\mu\nabla^\sigma \right)\delta_\nu^{\ \theta}+g_{\mu\nu}R^{\sigma\theta}-g_{\mu\nu}\nabla^\sigma\nabla^\theta -R_\mu{}^\sigma{}_\nu {}^\theta\\
&\quad+\left(2\Lambda-R-\Delta \right)\delta_{\mu}^{\ \sigma}\delta_{\nu}^{\ \theta}+\delta_{\mu}^{\ \sigma}\nabla^\theta\nabla_\nu\Big]\left[d-\frac{3\left(2+b\right)}{4}\right] \ .
\end{split}
\ee
It is clear that the full expression for the difference $S_{\mu\nu}\equiv B_{\mu\nu}-E_{\mu\nu}$ can become extremely complicated. Therefore, we focus on a specific example.

\subsection{$b=d=0$}
By imposing $b=d=0$, we also have $f=0$. Moreover, this implies $e=-3/2$ and:
\be 
\begin{split}
    f_D=-\frac{3}{4}\ ,\quad g_D=\frac{1}{2}\ .
\end{split}
\ee
Concerning the operators appearing in $B_{\mu\nu}$, we have $\Omega_{\mu\nu}=0$,
\be
\begin{split}
   \Theta_{\mu\nu}&=\frac{3}{2}\left(\nabla_\mu\nabla_\nu -g_{\mu\nu}\Delta\right)\ ,
\end{split}
\ee
and
\be
\begin{split}
   \Sigma_{\mu\nu}^{\sigma\theta}&= -\frac{3}{2}\Big[\left(R_\mu{}^\sigma+\nabla_\mu\nabla^\sigma \right)\delta_\nu^{\ \theta}+g_{\mu\nu}R^{\sigma\theta}-g_{\mu\nu}\nabla^\sigma\nabla^\theta -R_\mu{}^\sigma{}_\nu {}^\theta\\
&\quad+\left(2\Lambda-R-\Delta \right)\delta_{\mu}^{\ \sigma}\delta_{\nu}^{\ \theta}+\delta_{\mu}^{\ \sigma}\nabla^\theta\nabla_\nu\Big] \ .
\end{split}
\ee
Therefore, $B_{\mu\nu}$ takes the form:
\be
\begin{split}
   B_{\mu\nu}&=-\nabla^\sigma\nabla_\nu R_{\mu\sigma}+\nabla_\mu\nabla_\nu R+\Delta R_{\mu\nu}+R_\mu{}^\sigma{}_\nu {}^\theta R_{\sigma\theta}\\
&\quad-\nabla_\mu\nabla^\sigma R_{\sigma\nu}-g_{\mu\nu}\frac{1}{2}\Delta R+RR_{\mu\nu}-R_\mu{}^\sigma R_{\sigma\nu}-2\Lambda R_{\mu\nu}\\
 &\quad+\left(C-R_{\sigma\theta}R^{\sigma\theta}\right)g_{\mu\nu}+\frac{3}{4}\left(\nabla_\mu\nabla_\nu -g_{\mu\nu}\Delta\right)\nabla_\alpha\phi\nabla^\alpha\phi\\
    &\quad-\frac{3}{4}\Big[\left(R_\mu{}^\sigma+\nabla_\mu\nabla^\sigma \right)\delta_\nu^{\ \theta}+g_{\mu\nu}R^{\sigma\theta}-g_{\mu\nu}\nabla^\sigma\nabla^\theta -R_\mu{}^\sigma{}_\nu {}^\theta\\
&\quad+\left(2\Lambda-R-\Delta \right)\delta_{\mu}^{\ \sigma}\delta_{\nu}^{\ \theta}+\delta_{\mu}^{\ \sigma}\nabla^\theta\nabla_\nu\Big]\nabla_\sigma\phi\nabla_\theta\phi\ ,
\end{split}
\ee
The $E_{\mu\nu}$ flow source component is, instead:
\be
\begin{split}
    E_{\mu\nu}&=-\nabla_\mu\phi\nabla_\nu R-\frac{3}{4}\nabla_\mu\phi\nabla_\nu\left(\nabla\phi\right)^{2}-\frac{1}{2}\nabla_\mu\phi\nabla_\nu\Delta\phi\\
    &\quad-\nabla_\nu\phi\nabla_\mu R-\frac{3}{4}\nabla_\nu\phi\nabla_\mu\left(\nabla\phi\right)^{2}-\frac{1}{2}\nabla_\nu\phi\nabla_\mu\Delta\phi\\
    &\quad-g_{\mu\nu}m^2\phi\left[-R-\frac{3}{4}\left(\nabla\phi\right)^{2}-\frac{1}{2}\Delta\phi\right]\\
    &\quad+g_{\mu\nu}\left[\nabla^\alpha\phi\nabla_\alpha R+\frac{3}{4}\nabla^\alpha\phi\nabla_\alpha\left(\nabla\phi\right)^{2}+\frac{1}{2}\nabla^\alpha\phi\nabla_\alpha\Delta\phi\right]\\
    &\quad+\left(R_{\mu\nu}-\frac{1}{4}\nabla_\mu\phi\nabla_\nu\phi\right)\nabla_\alpha\phi\nabla^\alpha\phi+m^2\left(R_{\mu\nu}-\frac{1}{4}\nabla_\mu\phi\nabla_\nu\phi\right)\phi^2
\end{split}
\ee
Hence, the difference allows just for a few simplification and has the form:
\be 
\begin{split}
 S_{\mu\nu}&=-\nabla^\sigma\nabla_\nu R_{\mu\sigma}+\nabla_\mu\nabla_\nu R+\Delta R_{\mu\nu}+R_\mu{}^\sigma{}_\nu {}^\theta R_{\sigma\theta}\\
&\quad-\nabla_\mu\nabla^\sigma R_{\sigma\nu}-g_{\mu\nu}\frac{1}{2}\Delta R+RR_{\mu\nu}-R_\mu{}^\sigma R_{\sigma\nu}-2\Lambda R_{\mu\nu}\\
 &\quad+\left(C-R_{\sigma\theta}R^{\sigma\theta}\right)g_{\mu\nu}+\frac{3}{4}\left(\nabla_\mu\nabla_\nu -g_{\mu\nu}\Delta\right)\nabla_\alpha\phi\nabla^\alpha\phi\\
    &\quad-\frac{3}{4}\Big[\left(R_\mu{}^\sigma+\nabla_\mu\nabla^\sigma \right)\delta_\nu^{\ \theta}+g_{\mu\nu}R^{\sigma\theta}-g_{\mu\nu}\nabla^\sigma\nabla^\theta -R_\mu{}^\sigma{}_\nu {}^\theta\\
&\quad+\left(2\Lambda-R-\Delta \right)\delta_{\mu}^{\ \sigma}\delta_{\nu}^{\ \theta}+\delta_{\mu}^{\ \sigma}\nabla^\theta\nabla_\nu\Big]\nabla_\sigma\phi\nabla_\theta\phi\\   
&\quad+\nabla_\mu\phi\nabla_\nu R+\frac{3}{4}\nabla_\mu\phi\nabla_\nu\left(\nabla\phi\right)^{2}+\frac{1}{2}\nabla_\mu\phi\nabla_\nu\Delta\phi\\
    &\quad+\nabla_\nu\phi\nabla_\mu R+\frac{3}{4}\nabla_\nu\phi\nabla_\mu\left(\nabla\phi\right)^{2}+\frac{1}{2}\nabla_\nu\phi\nabla_\mu\Delta\phi\\
    &\quad+g_{\mu\nu}m^2\phi\left[-R-\frac{3}{4}\left(\nabla\phi\right)^{2}-\frac{1}{2}\Delta\phi\right]\\
    &\quad-g_{\mu\nu}\left[\nabla^\alpha\phi\nabla_\alpha R+\frac{3}{4}\nabla^\alpha\phi\nabla_\alpha\left(\nabla\phi\right)^{2}+\frac{1}{2}\nabla^\alpha\phi\nabla_\alpha\Delta\phi\right]\\
    &\quad-\left(R_{\mu\nu}-\frac{1}{4}\nabla_\mu\phi\nabla_\nu\phi\right)\left(\nabla_\alpha\phi\nabla^\alpha\phi+m^2\phi^2\right)\ .
\end{split}
\ee
